# Supplementary material for: On a Utilitarian Approach to Privacy Preserving Text Generation
Source: arXiv:2104.11838 source file (2021-04-23)
Supplement: Supplementary file 1 [file appendix.tex]

\section{Appendix: additional experiments}
